# Supplementary material for: Quantum correlations at infinite temperature: the dynamical Nagaoka effect
Source: arXiv:1703.09231 ancillary file (2017-03-27)
Supplement: Supplementary file 1 [file supplementary.pdf]

# Supplementary material for "Dynamical Nagaoka effect in an infinite temperature spin environment"

Márton Kanász-Nagy,[1] Izabella Lovas,[2] Fabian Grusdt,[1] Daniel Greif,[1] Markus Greiner,[1] and Eugene A. Demler[1]

[1]*Department of Physics, Harvard University, Cambridge MA 02138, United States*
[2]*MTA-BME Exotic Quantum Phases "Momentum" Research Group and Department of Theoretical Physics, Budapest University of Technology and Economics, 1111 Budapest, Hungary*

## I. MODELING EXPERIMENTAL ERROR

Quantum gas microscope experiments take individual measurements of the spin configuration on the lattice, and the thermal average is evaluated by averaging over many experimental runs. In the infinite temperature spin environment, each spin takes on one of the $\mathcal{N}$ spin states with equal probability. Therefore, after $K$ measurements, the experimental error of the spin correlations is proportional to $K^{-1/2}$. In order to reduce experimental error, one can also make use of the reflection and four-fold rotation symmetries of the two-dimensional lattice, and average the spin correlations according to these symmetries. We illustrate the role of experimental error, by starting simulations from $K$ random initial spin configurations $|\Gamma_i\rangle$ in a spin $S = 1/2$ system. Instead of evaluating the spin average exactly as we did in the main text, we average over only these configurations $C_{jl}(t) \approx \frac{1}{K}\sum_{i=1}^{K}\langle\Gamma_i|c_o\, e^{iHt}\, S_j^z S_l^z\, e^{-iHt} c_o^\dagger|\Gamma_i\rangle$. Fig. S1 shows the spin correlations of the hole after symmetry averaging. We obtain good signal-to-noise ratio already after $K = 500$ runs. The details of the quantum Monte Carlo procedure performing finite number of spin averaging is described in Methods.

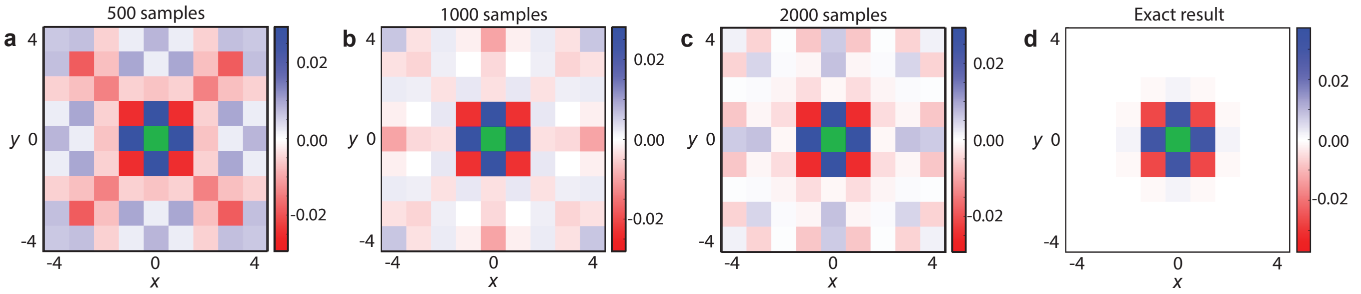


FIG. S1. **Simulation of spin correlations after a finite number of experimental runs.** Spin correlations $C_{jl}(t)$ measured after time evolution of $t = 1.2$ in a spin $S = 1/2$ system. The reference site $j$ is chosen to be the origin, whereas the coordinates of the lattice correspond to site $l$. The spin correlations are averaged over the four-fold rotational symmetry and over all reflection symmetries of the lattice to obtain better signal to noise ratio. **a**, **b**, **c** and **d** represent averaging over 500, 1000, 2000 and all initial spin states, respectively.

## II. BREAKDOWN OF PERTURBATION THEORY TO FINITE ORDERS

Due to the degeneracy of the spin environment, perturbation theory of the time evolution up to any finite order in time breaks down, as we discussed in the main text [1]. Therefore, the expansion of the time evolution $e^{-iHt} = \sum_{n=0}^{\infty}\frac{(-it)^n}{n!}H^n$ needs to be summed up to infinite order. We perform the summation numerically by sampling the paths of the hole using a quantum Monte Carlo procedure [2]. This method falls into the family of stochastic series expansion quantum Monte Carlo techniques [3]. As we discussed in the main text, the paths are chosen according to a Poisson distribution of mean $zt$, where $z = 4$ is the coordination number of the lattice. Fig S2 a shows the distribution of paths at different times. Whereas the average length of paths is $zt$, one needs to take into account significantly shorter and longer paths as well to ensure convergence. Truncating the series at any finite order, and thereby neglecting the contribution of long paths leads to the divergence of the time evolution of the spin correlations $C_{jl}(t)$ at long enough times, as we show in Fig S2 b.

## III. ANALYTICAL SOLUTION OF HOLE PROPAGATION ON THE BETHE LATTICE

In this section we derive an analytical expression for the wave function of the hole on the Bethe lattice. By expanding the propagator into Taylor series, we can express the time evolution of the wave function at site $j$, $\psi_j^{\rm site}$, in terms of random walk

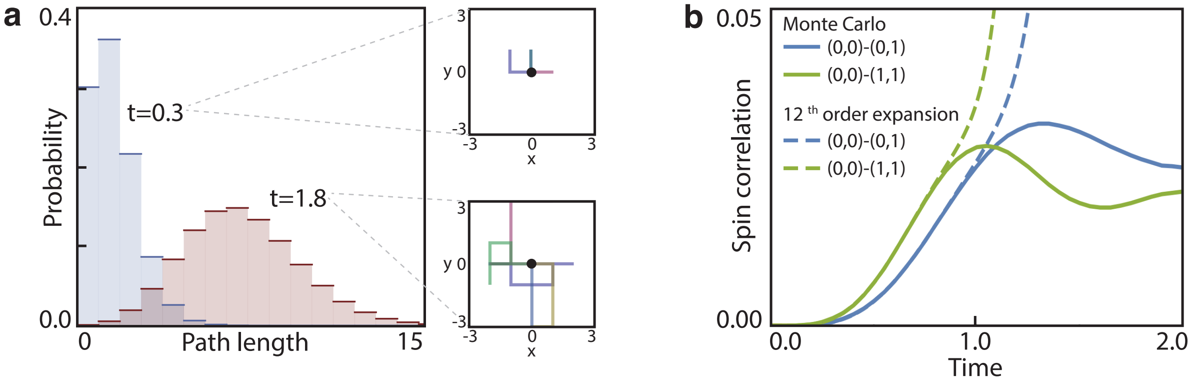


FIG. S2. **Quantum Monte Carlo versus finite order perturbation theory. a,** Distribution of the path lengths in the quantum Monte Carlo algorithm at different times. The panels show five different examples of random paths at these times. **b,** Comparison of spin correlations results using perturbation theory to $12^{\text{th}}$ order in time (dashed lines) versus the quantum Monte Carlo procedure presented in the main text (full lines). Blue and green lines denote correlations between sites $(0,0)-(0,1)$ and $(0,0)-(1,1)$, respectively.

paths ending at $j$. This expansion leads to

$$\psi_j^{\text{site}}(t) = \sum_{k=0}^{\infty} \frac{(it)^k}{k!} N_k^{(j)}, \tag{1}$$

where $N_k^{(j)}$ denotes the number of random walks of length $k$, starting from the origin and ending at site $j$. In order to evaluate $N_k^{(j)}$, let us redraw the Bethe lattice in a way slightly different from Fig. 4a. As the Bethe lattice is infinite, and each node has a coordination number 4, we can relabel its levels in such a way that all sites have three downward and one upward edges (see Fig. S3). To avoid confusion with the original lattice, we will refer to these relabelled levels as the *depth* of sites in the graph. Even though this rearranging of vertices does not reflect the symmetry of the wave function, it has the advantage of assigning the same number of upward and downward edges to each node, whereas in Fig. 4 in the main text the origin was a special point with four downward edges. This new symmetry will be convenient for counting the number of random walks $N_k^{(j)}$.

The depth of the origin is chosen to be 0. Consider a site $j$ in the lower branch of the tree, starting from the origin, as in Fig. S3. It is enough to calculate the wave function for sites positioned like this, because the wave function of every remaining site follows from the (now somewhat hidden) symmetry of $\psi$. The depth of site $j$ will be denoted by $d_j$.

To calculate the number of random walks $N_k^{(j)}$, let us group the different trajectories ending at site $j$ according to the lowest depth they reach in the Bethe tree, $-n$ (with $n \geq 0$, since the walk starts from the origin with depth 0). As a first step, we calculate the number of random walks starting from the origin, reaching depth $-n$ as a deepest position, and ending at depth $d_j$. Such random trajectories have to consist of $d_j + 2n + 2m$ steps with some $m \geq 0$. We will now determine the number of random walks for a fixed step number $d_j + 2n + 2m$.

For ending up at depth $d_j$, the walker has to take $d_j + n + m$ downward and $n + m$ upward steps. The number of possible up-down sequences is $\binom{d_j+2n+2m}{n+m}$, but not all sequences correspond to random walks with lowest depth $-n$. First we count the number of sequences reaching depth $-n$ (but maybe lower depths as well), relying on the reflection principle for random walks.

Consider an up-down sequence of length $d_j + 2n + 2m$, reaching depth $-n$ and ending at depth $d_j$ (see Fig. S4). Look for the point where the walker visits depth $-n$ for the last time, and reflect the section of the sequence after this point to the level of depth $-n$ (see Fig. S4). This way we get a sequence ending at depth $-d_j - 2n$. The mapping described above is a bijective map between sequences reaching depth $-n$ and ending at depth $d_j$, and sequences ending at depth $-d_j - 2n$, so it is enough to calculate the number of the latter random walks. Such sequences involve $m$ downward and $d_j + 2n + m$ upward steps, giving $\binom{d_j+2n+2m}{m}$ possibilities.

So far we calculated the number of up-down sequences visiting depth $-n$, but these random walks may reach lower depths as well. In order to determine the number of sequences with $-n$ as their lowest depth, we have to subtract from $\binom{d_j+2n+2m}{m}$ the number of random walks reaching depth $-n-1$. Repeating the argument above, this number is equal to the number of sequences ending at depth $-d_j - 2(n+1)$, giving $\binom{d_j+2n+2m}{m-1}$ possibilities. Subtracting this from the number of up-down sequences visiting $-n$, we get the total number of sequences ending at $d_j$, with lowest depth $-n$,

$$\binom{d_j + 2n + m}{m} - \binom{d_j + 2n + m}{m-1} = (d_j + 2n + 1)\frac{(d_j + 2n + 2m)!}{m!(d_j + 2n + m + 1)!}.$$

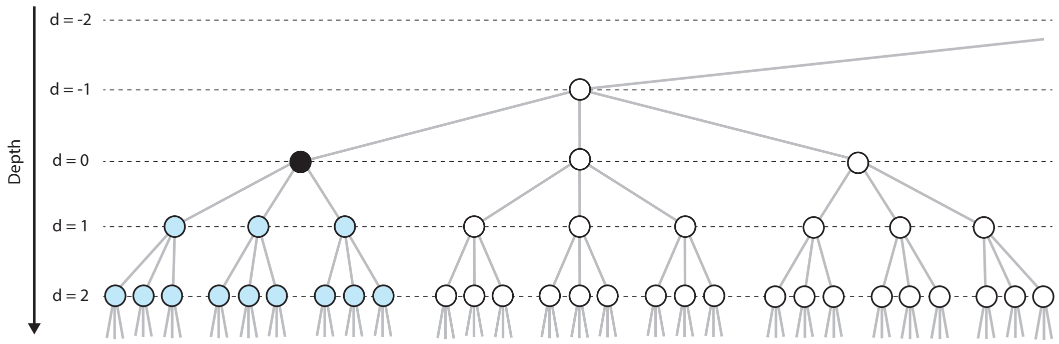


FIG. S3. **Bethe lattice redrawn with three downward edges for each site.** Levels are relabelled according to their depth $d$ in the graph (dashed lines), with the origin (black dot) lying at depth $d = 0$. Due to symmetry, it is enough to calculate the wave function for the sites in the branch below the origin (blue dots). Random walks start from the origin, and they are grouped according to the lowest depth they reach in the graph. For example, a walk visiting depth $d = -1$, but not reaching depth $d = -2$, can end at any of the 9 sites of depth $d = 1$ in the figure with equal probability. Other sites at depth $d = 1$ (not shown here) can not be reached by this walker.

Each one of these up-down sequences involves $d_j + n + m$ downward and $n + m$ upward steps. Every site has 3 downward edges, so the walker can choose between 3 directions for each downward step, leading to an additional factor of $3^{d_j+n+m}$ in the number of random walks. These walks all end at depth $d_j$, but we only want to take into account those which end at site $j$. A random walk starting from the origin and reaching lowest depth $-n$ can end at $3^{n+d_j}$ different sites at depth $d_j$ (see Fig. S3). By symmetry each of these endpoints has equal probability, leading to the final result

$$N_k^{(j)} = \sum_{n=0}^{\infty}\sum_{m=0}^{\infty} \delta_{k,d_j+2n+2m}\,\frac{1}{3^{d_j+n}}\,3^{d_j+n+m}\,(d_j+2n+1)\frac{(d_j+2n+2m)!}{m!(d_j+2n+m+1)!}.$$

Substituting this result into Eq. (1), and summing over all possible $n$ and $m$ values gives

$$\begin{aligned}\psi_j^{\text{site}}(t) &= \sum_{n=0}^{\infty}\sum_{m=0}^{\infty} 3^m\,\frac{(i\,t)^{d_j+2n+2m}}{(d_j+2n+2m)!}\,\frac{(d_j+2n+2m)!}{m!\,(d_j+2n+m+1)!}\,(d_j+2n+1)\\ &= \frac{i^{d_j}}{3^{d_j/2}}\sum_{n=0}^{\infty}(-1)^n\,\frac{d_j+2n+1}{3^n}\,\frac{J_{d_j+2n+1}(2\sqrt{3}\,t)}{\sqrt{3}\,t},\end{aligned}$$

with $J_{d_j+2n+1}$ denoting the Bessel function of the first kind.

If we again draw the Bethe lattice as in Fig. 4 in the main text, the wave function only depends on the level index $l$. Based on the previous expression, we arrive at the analytical result

$$\psi_l(t) = \frac{i^l}{3^{l/2}}\sum_{n=0}^{\infty}(-1)^n\,\frac{l+2n+1}{3^n}\,\frac{J_{l+2n+1}(2\sqrt{3}\,t)}{\sqrt{3}\,t}.$$

## IV. BALLISTIC PROPAGATION ON THE BETHE LATTICE

In this section we show numerically that the propagation of the hole on the Bethe lattice is ballistic. The average level index of the hole,

$$\bar{l}(t) = \sum_{l=0}^{\infty} l\,N_l\,|\psi_l(t)|^2,$$

is plotted as a function of propagation time $t$ in Fig S5. Here $N_l$ denotes the number of sites at level $l$ of the Bethe lattice (see Fig. 4 in the main text). The average level index increases linearly in time, confirming ballistic propagation with

$$\bar{l}(t) \sim 2.73\,t$$

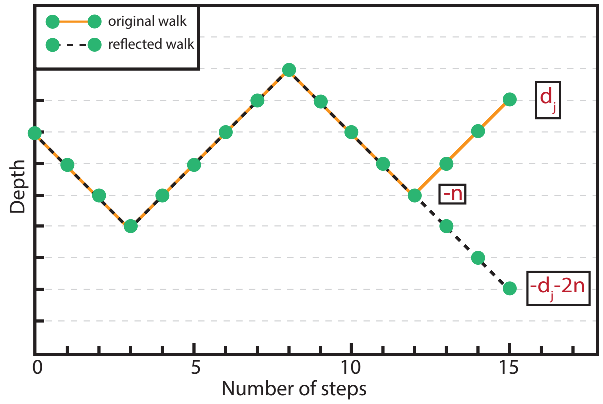


FIG. S4. **Reflection principle for random walks.** Bijective mapping between random up-down sequences ending at depth $d_j$ while visiting depth $-n$, and sequences ending at depth $-d_j - 2n$. Find the point when the walker headed to depth $d_j$ visits a site at depth $-n$ for the last time, and reflect the remaining section of the walk to the level of depth $-n$. The new walk will end at depth $-d_j - 2n$. For illustration we used $d_j = 1$ and $n = 2$.

for long times $t \gg 1$.

After mapping the Bethe lattice to the square lattice, the RMS distance of the sites at level $l$ grows as $d_l \sim \sqrt{2\,l}$ for large distances $l \gg 1$ (see Methods). Due to this relation, the ballistic propagation found above gives rise to a diffusive behavior on the square lattice, with diffusion constant $D_{\text{Bethe}} = 2.73$.

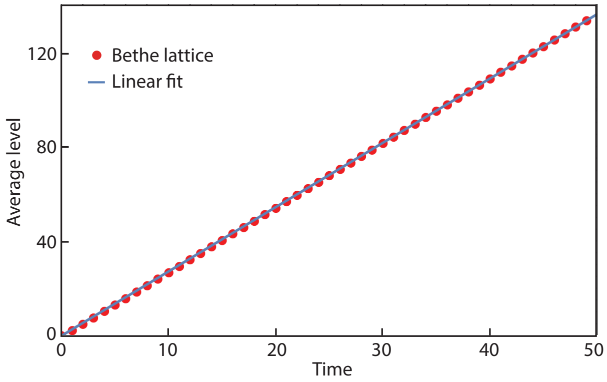


FIG. S5. **Ballistic propagation on the Bethe lattice.** Average level index of the hole $\langle l \rangle$ as a function of propagation time $t$ (symbols), compared to ballistic propagation $\langle l \rangle = 2.73\,t$ (solid line). Ballistic propagation on the Bethe lattice corresponds to diffusive behavior on the square lattice with diffusion constant $D_{\text{Bethe}} = 2.73$.


[1] Esterling, D. M. & Lange, R. V. Hubbard model. i. degeneracy in the atomic light. *Phys. Rev. B* **1**, 2231–2237 (1970). URL `http://link.aps.org/doi/10.1103/PhysRevB.1.2231`.

[2] Carlström, J., Prokof'ev, N. & Svistunov, B. Quantum walk in degenerate spin environments. *Phys. Rev. Lett.* **116**, 247202 (2016). URL `http://link.aps.org/doi/10.1103/PhysRevLett.116.247202`.

[3] Sandvik, A. W. & Kurkijärvi, J. Quantum monte carlo simulation method for spin systems. *Phys. Rev. B* **43**, 5950–5961 (1991). URL `http://link.aps.org/doi/10.1103/PhysRevB.43.5950`.
